# Supplementary material for: Spatio-Temporal Hybrid Graph Convolutional Network for Traffic Forecasting in Telecommunication Networks
Source: arXiv:2009.09849 source file (2020-09-17)
Supplement: Supplementary file 1 [file 08.appendix.tex]

\section{Appendix}

\begin{comment}
\begin{appendices}
\chapter{Some Appendix}
The contents...
\end{appendices}
\end{comment}
